# Supplementary material for: Understanding or Manipulation: Rethinking Online Performance Gains of Modern Recommender Systems
Source: arXiv:2210.05662 source file (2023-12-18)
Supplement: Supplementary file 1 [file 9-appendix.tex]

\appendix
